# Supplementary material for: Sequential Attention for Feature Selection
Source: arXiv:2209.14881 source file (2023-04-25)
Supplement: Supplementary file 1 [file appendix_seql_omp.tex]

\subsection{Sequential LASSO and OMP}\label{sec:seql-omp-exp}

Our theoretical analysis in Section \ref{sec:seql-omp} predicts that both the Sequential LASSO and OMP are good feature selection algorithms that are equivalent to Sequential Attention, and thus should perform comparably to our results for Sequential Attention. In this section, we evaluate the performance of Sequential LASSO and OMP and compare it to that of Sequential Attention.

For Sequential LASSO, we observe in Figures \ref{fig:seql-accuracy} and \ref{fig:seql} that while Sequential LASSO marginally outperforms Sequential Attention in some cases, Sequential Attention generally achieves similar or better accuracies than Sequential LASSO. Furthermore, Sequential LASSO requires a tuning of the regularization parameter to be competitive with Sequenital Attention, whereas we do not require additional hyperparameters for Sequential Attention. We also show in Figure \ref{fig:gl-accuracy} the corresponding accuracies achieved by Group LASSO \cite{SCHU2017}, which is the non-sequential variant of the Sequential LASSO.

\begin{figure}[H]
\caption{Accuracies achieved by Sequential LASSO with various regularization parameters.}
\centering
\begin{tabular}{ c c c c c c c c c } 
\toprule
Dataset & 0 & $10^{-5}$ & $10^{-4}$ & $10^{-3}$ & $10^{-2}$ & $10^{-1}$ & $1$ & $10$ \\
\midrule
Mice & 0.968 & \textbf{0.972} & \textbf{0.972} & \textbf{0.972} & 0.958 & 0.875 & 0.889 & 0.838 \\
MNIST & 0.331 & 0.900 & 0.947 & 0.953 & \textbf{0.963} & 0.946 & 0.434 & 0.809 \\
MNIST-Fashion & 0.332 & 0.618 & 0.789 & 0.844 & \textbf{0.856} & 0.807 & 0.772 & 0.811 \\
ISOLET & 0.687 & 0.689 & 0.818 & 0.887 & \textbf{0.920} & 0.812 & 0.863 & 0.84 \\
COIL-20 & 0.844 & 0.944 & 0.962 & \textbf{0.979} & 0.965 & 0.931 & 0.976 & 0.951 \\
Activity & 0.898 & 0.906 & 0.912 & 0.930 & 0.930 & 0.883 & 0.792 & \textbf{0.931} \\
\bottomrule
\end{tabular}
\label{fig:seql-accuracy}
\end{figure}

\begin{figure}[H]
\caption{Accuracies achieved by Group LASSO \cite{SCHU2017} with various regularization parameters.}
\centering
\begin{tabular}{ c c c c c c c c c } 
\toprule
Dataset & 0 & $10^{-5}$ & $10^{-4}$ & $10^{-3}$ & $10^{-2}$ & $10^{-1}$ & $1$ & $10$ \\
\midrule
Mice & 0.968 & 0.972 & 0.972 & \textbf{0.977} & 0.963 & 0.903 & 0 & 0.898 \\
MNIST & 0.323 & 0.921 & 0.932 & \textbf{0.942} & 0.934 & 0.936 & 0.863 & 0.798 \\
MNIST-Fashion & 0.323 & 0.571 & 0.74 & 0.829 & \textbf{0.839} & 0.836 & 0.798 & 0.805 \\
ISOLET & 0.686 & 0.697 & 0.831 & 0.868 & \textbf{0.914} & 0.794 & 0.855 & 0.879 \\
COIL-20 & 0.844 & 0.958 & 0.965 & 0.972 & \textbf{0.983} & 0.969 & 0.965 & 0.972 \\
Activity & 0.898 & 0.906 & 0.916 & 0.923 & \textbf{0.940} & 0.884 & 0.838 & 0.848 \\
\bottomrule
\end{tabular}
\label{fig:gl-accuracy}
\end{figure}

\begin{figure}[ht]
\centering
\includegraphics[scale=0.4]{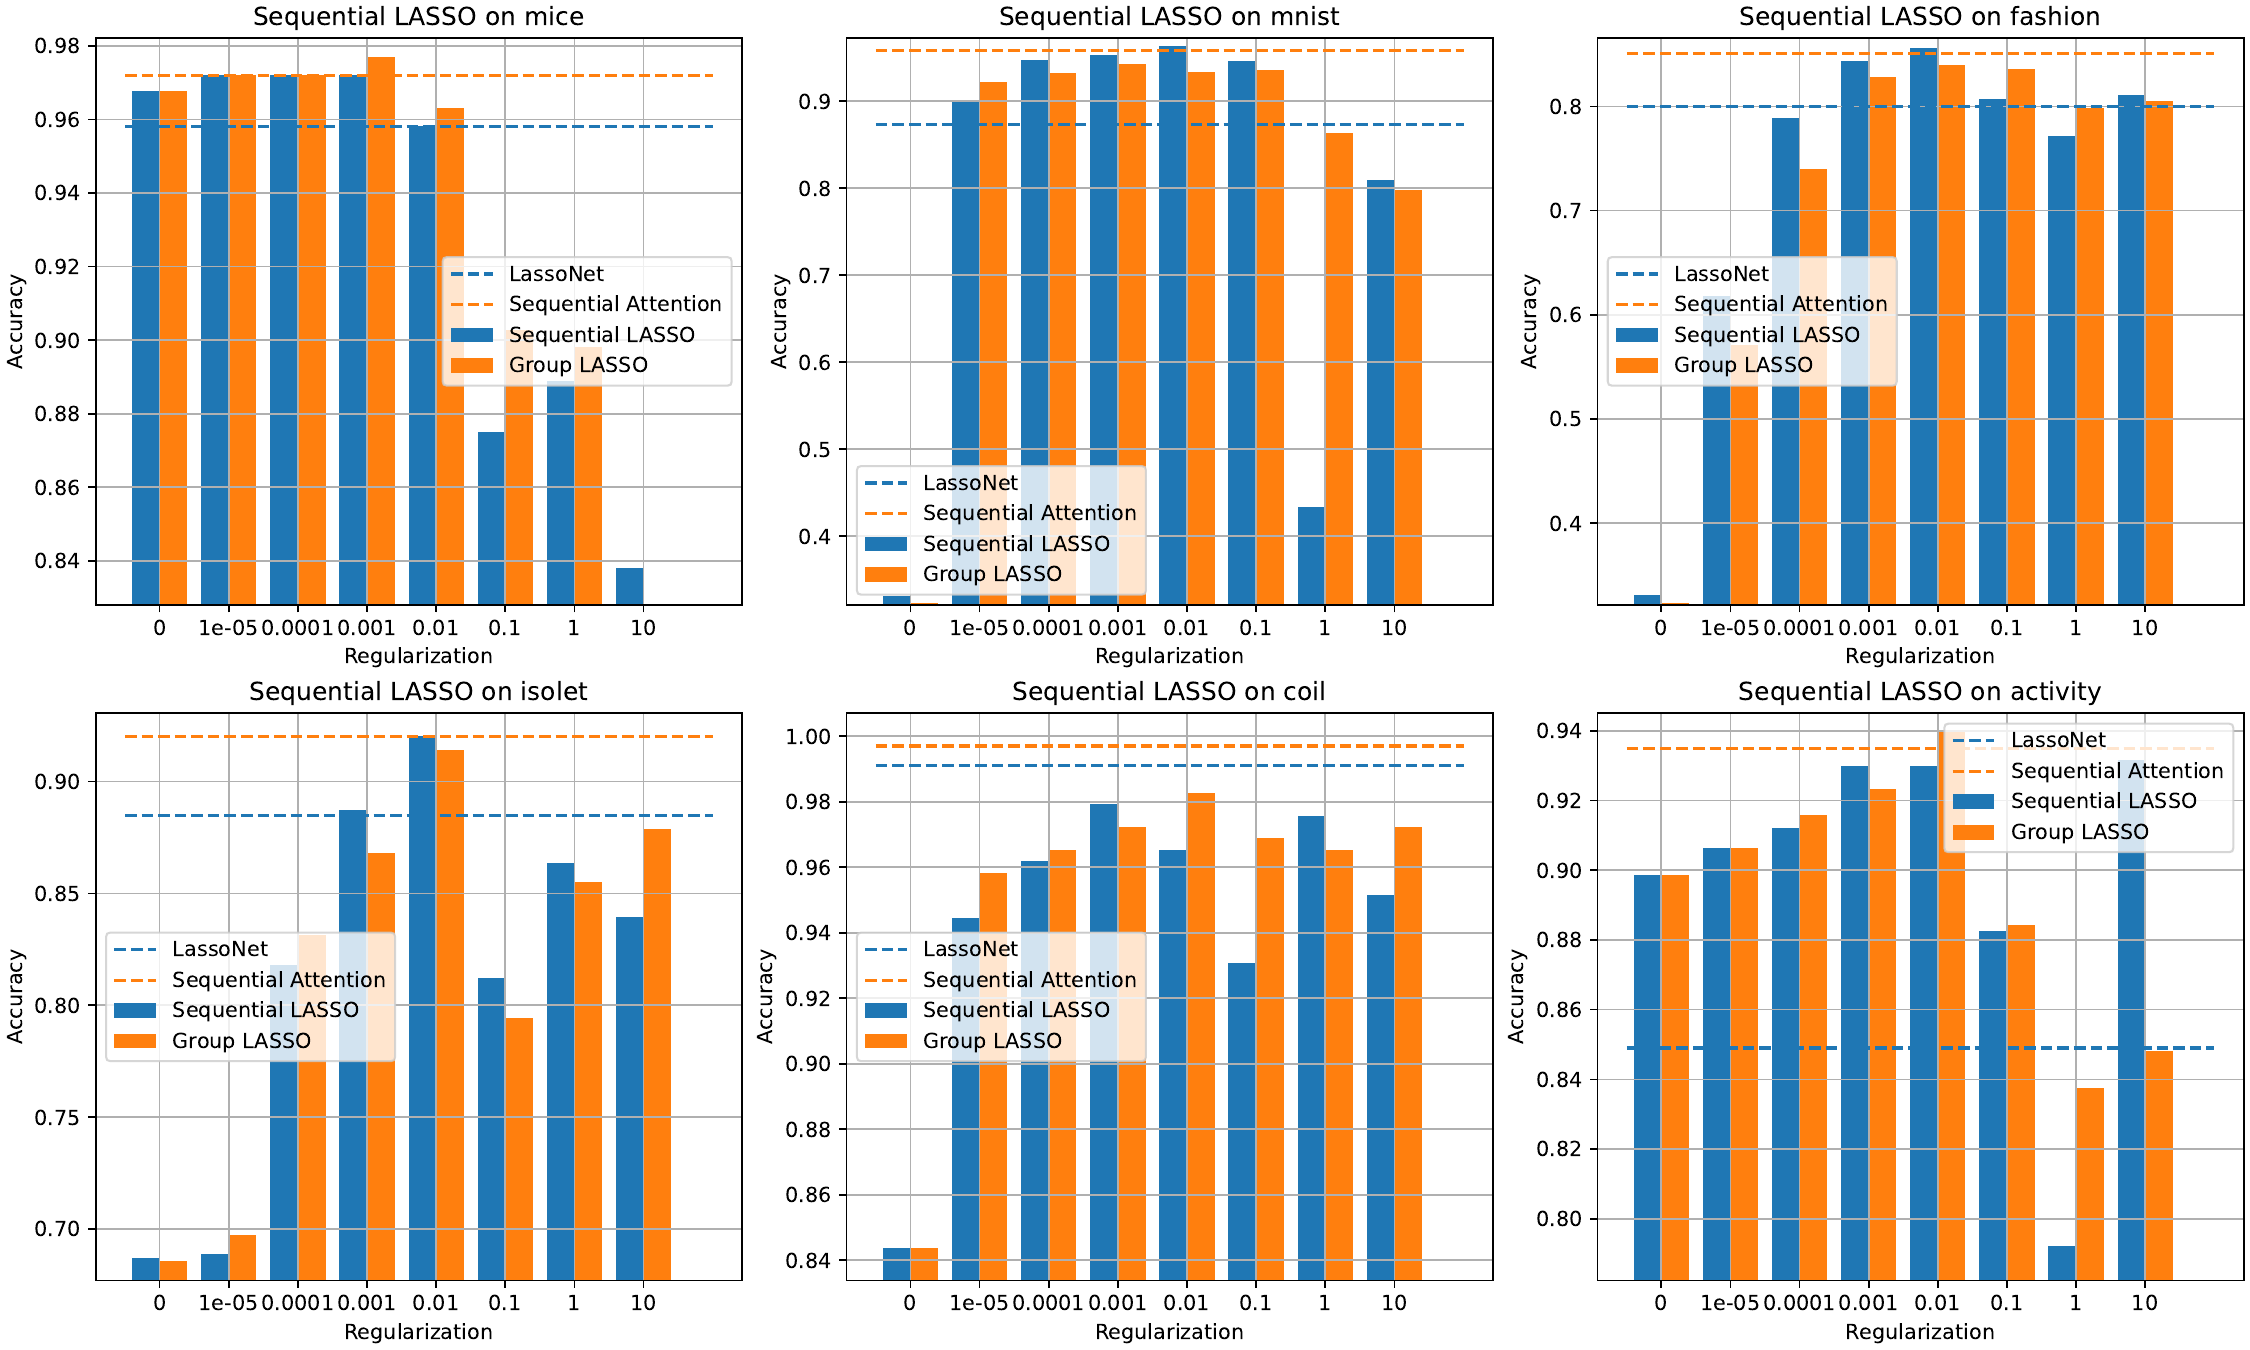}
\caption{\textbf{Sequential and Group LASSO experiments.} The $x$ axis ranges over various regularization parameters in powers of 10, while the $y$ axis shows the corresponding accuracy. While Sequential LASSO marginally outperforms Sequential Attention in some cases, Sequential Attention generally achieves similar or better accuracies than Sequential LASSO.}
\label{fig:seql}
\end{figure}

We also consider a natural generalization of the OMP for neural networks by viewing it as a generalized linear model for any fixing of the neural network weights and using the OMP for generalized linear models as suggested in \cite{EKDN2018}, where the gradient serves as the marginal feature importance signal. The accuracies are reported in Figure \ref{fig:omp-accuracy}. Perhaps surprisingly, the performance of OMP pales in comparison to Sequential LASSO and Sequential Attention. 

\begin{figure}[H]
\caption{Accuracies achieved by OMP \cite{PRK1993, EKDN2018}.}
\centering
\begin{tabular}{ c c } 
\toprule
Dataset & OMP \\
\midrule
Mice & 0.472 \\
MNIST & 0.917 \\
MNIST-Fashion & 0.711 \\
ISOLET & 0.572 \\
COIL-20 & 0.951 \\
Activity & 0.910 \\
\bottomrule
\end{tabular}
\label{fig:omp-accuracy}
\end{figure}
